# Supplementary material for: New generation of effective core potentials from correlated calculations: 2nd row elements
Source: arXiv:1805.00607 ancillary file (2018-09-07)
Supplement: Supplementary file 1 [file supplement.pdf]

# Supplementary Material: A new generation of effective core potentials from correlated calculations: 2nd row elements

M. Chandler Bennett[1,2], Guangming Wang[1], Abdulgani Annaberdiyev[1],
Cody A. Melton[1,2], Luke Shulenburger[2], and Lubos Mitas[1]

*1) Department of Physics,*
*North Carolina State University, Raleigh,*
*North Carolina 27695-8202, USA*
*and*
*2) Sandia National Laboratories,*
*Albuquerque, New Mexico 87123, USA*

(Dated: September 7, 2018)

PACS numbers:

## I. ATOMIC DATA

In Tables I-XVI, we show total energy components from various states of each of our ECPs from CCSD(T) calculations. All atomic calculations utilized the uncontracted aug-cc-pCVnZ basis sets where $n = \{T, Q, 5\}$. Each energy component, Hartree-Fock (SCF) and correlation, is extrapolated to the complete basis set (CBS) limit with the parameterized functions

$$E^{\text{SCF}}(n) = E^{\text{SCF}}_{\text{CBS}} + A \exp\big( - Bn\big) \tag{1}$$

and

$$E^{\text{Correlation}}(n) = E^{\text{Correlation}}_{\text{CBS}} + \frac{C}{(n+3/8)^3} + \frac{D}{(n+3/8)^5}\,, \tag{2}$$

respectively. The variables $A$, $B$, $C$ , $D$, $E^{\text{SCF}}_{\text{CBS}}$ and $E^{\text{Correlation}}_{\text{CBS}}$ are fitting parameters.

TABLE I: Total energy components of various states of the Na atom using our ccECP[Ne]

| SCF | | T | Q | 5 | CBS |
|---|---|---|---|---|---|
| [Ne] $3s^1$ | $^2S$ | -0.186167 | -0.186202 | -0.186202 | -0.186203 |
| [Ne] $3s^2$ | $^1S$ | -0.182241 | -0.182308 | -0.182308 | -0.182313 |
| Correlation | | T | Q | 5 | CBS |
| [Ne] $3s^1$ | $^2S$ | | | | |
| [Ne] $3s^2$ | $^1S$ | -0.024246 | -0.024271 | -0.02428 | -0.02429 |

TABLE II: Total energy components of various states of the Na atom using our ccECP[He]

| SCF | | T | Q | 5 | CBS |
|---|---|---|---|---|---|
| [Ne] $3s^1$ | $^2S$ | -47.355004 | -47.356999 | -47.357015 | -47.357015 |
| [Ne] | $^1S$ | -47.172935 | -47.174928 | -47.174944 | -47.174944 |
| [Ne] $3s^2$ | $^1S$ | -47.351159 | -47.353181 | -47.353197 | -47.353197 |
| Correlation | | T | Q | 5 | CBS |
| [Ne] $3s^1$ | $^2S$ | -0.278836 | -0.304079 | -0.313965 | -0.325551 |
| [Ne] | $^1S$ | -0.273772 | -0.298106 | -0.307423 | -0.318131 |
| [Ne] $3s^2$ | $^1S$ | -0.302615 | -0.327913 | -0.337849 | -0.349521 |

TABLE III: Total energy components of various states of the Mg atom using our ccECP[Ne]

| SCF | | T | Q | 5 | CBS |
|---|---|---|---|---|---|
| [Ne] $3s^2$ | $^1S$ | -0.788370 | -0.788345 | -0.788370 | -0.788370 |
| [Ne] $3s^1$ | $^2S$ | -0.544766 | -0.544744 | -0.544763 | -0.544763 |
| Correlation | | T | Q | 5 | CBS |
| [Ne] $3s^2$ | $^1S$ | -0.034907 | -0.034994 | -0.035031 | -0.035077 |
| [Ne] $3s^1$ | $^2S$ | | | | |

TABLE IV: Total energy components of various states of the Mg atom using our ccECP[He]

| SCF | | T | Q | 5 | CBS |
|---|---|---|---|---|---|
| [Ne] $3s^2$ | $^1S$ | -62.927052 | -62.927327 | -62.927412 | -62.927451 |
| [Ne] | $^1S$ | -62.142427 | -62.142705 | -62.142790 | -62.142828 |
| [Ne] $3s^1$ | $^2S$ | -62.684058 | -62.684333 | -62.684414 | -62.684447 |
| Correlation | | T | Q | 5 | CBS |
| [Ne] $3s^2$ | $^1S$ | -0.315920 | -0.342027 | -0.352077 | -0.363681 |
| [Ne] | $^1S$ | -0.270494 | -0.294814 | -0.304048 | -0.314584 |
| [Ne] $3s^1$ | $^2S$ | -0.279223 | -0.304733 | -0.314498 | -0.325718 |

TABLE V: Total energy components of various states of the Al atom using our ccECP[Ne]

| SCF | | T | Q | 5 | CBS |
|---|---|---|---|---|---|
| [Ne] $3s^2 3p^1$ | $^2P$ | -1.876699 | -1.876990 | -1.876973 | -1.876999 |
| [Ne] $3s^1$ | $^2S$ | -1.030941 | -1.030946 | -1.030933 | -1.030949 |
| [Ne] $3s^2$ | $^1S$ | -1.674980 | -1.675006 | -1.674996 | -1.675010 |
| [Ne] $3s^2 3p^2$ | $^3P$ | -1.878405 | -1.878616 | -1.878601 | -1.878623 |
| Correlation | | T | Q | 5 | CBS |
| [Ne] $3s^2 3p^1$ | $^2P$ | -0.058680 | -0.059582 | -0.059783 | -0.059869 |
| [Ne] $3s^1$ | $^2S$ | | | | |
| [Ne] $3s^2$ | $^1S$ | -0.041715 | -0.042057 | -0.042137 | -0.042175 |
| [Ne] $3s^2 3p^2$ | $^3P$ | -0.072470 | -0.073840 | -0.074155 | -0.074305 |

TABLE VI: Total energy components of various states of the Al atom using our ccECP[He]

| SCF | | T | Q | 5 | CBS |
|---|---|---|---|---|---|
| [Ne] $3s^2 3p^1$ | $^2P$ | -80.990584 | -80.992910 | -80.993046 | -80.993054 |
| [Ne] | $^1S$ | -79.112214 | -79.114296 | -79.114427 | -79.114435 |
| [Ne] $3s^1$ | $^2S$ | -80.144308 | -80.146349 | -80.146470 | -80.146478 |
| [Ne] $3s^2$ | $^1S$ | -80.789130 | -80.791175 | -80.791301 | -80.791309 |
| [Ne] $3s^2 3p^2$ | $^3P$ | -80.992087 | -80.994343 | -80.994480 | -80.994489 |
| Correlation | | T | Q | 5 | CBS |
| [Ne] $3s^2 3p^1$ | $^2P$ | -0.305640 | -0.355044 | -0.373996 | -0.395813 |
| [Ne] | $^1S$ | -0.231923 | -0.278793 | -0.297044 | -0.318327 |
| [Ne] $3s^1$ | $^2S$ | -0.243946 | -0.291640 | -0.310130 | -0.331614 |
| [Ne] $3s^2$ | $^1S$ | -0.289386 | -0.338035 | -0.356793 | -0.378485 |
| [Ne] $3s^2 3p^2$ | $^3P$ | -0.319051 | -0.368907 | -0.387970 | -0.409853 |

TABLE VII: Total energy components of various states of the Si atom using our ccECP[Ne]

| SCF | | T | Q | 5 | CBS |
|---|---|---|---|---|---|
| [Ne] $3s^2 3p^2$ | $^3P$ | -3.671951 | -3.672403 | -3.672394 | -3.672423 |
| [Ne] $3s^1$ | $^2S$ | -1.639761 | -1.639759 | -1.639758 | -1.639762 |
| [Ne] $3s^2$ | $^1S$ | -2.813851 | -2.813866 | -2.813855 | -2.813870 |
| [Ne] $3s^2 3p^1$ | $^2P$ | -3.390158 | -3.390719 | -3.390718 | -3.390749 |
| [Ne] $3s^2 3p^3$ | $^4S$ | -3.707923 | -3.708178 | -3.708158 | -3.708187 |
| Correlation | | T | Q | 5 | CBS |
| [Ne] $3s^2 3p^2$ | $^3P$ | -0.085857 | -0.087646 | -0.088188 | -0.088666 |
| [Ne] $3s^1$ | $^2S$ | | | | |
| [Ne] $3s^2$ | $^1S$ | -0.047828 | -0.048152 | -0.048263 | -0.048376 |
| [Ne] $3s^2 3p^1$ | $^2P$ | -0.068862 | -0.069816 | -0.070130 | -0.070437 |
| [Ne] $3s^2 3p^3$ | $^4S$ | -0.100941 | -0.103501 | -0.104256 | -0.104894 |

TABLE VIII: Total energy components of various states of the Si atom using our ccECP[He]

| SCF | | T | Q | 5 | CBS |
|---|---|---|---|---|---|
| [Ne] $3s^2 3p^2$ | $^3P$ | -101.622367 | -101.625367 | -101.625788 | -101.625857 |
| [Ne] | $^1S$ | -97.946272 | -97.948793 | -97.949212 | -97.949296 |
| [Ne] $3s^1$ | $^2S$ | -99.589327 | -99.591835 | -99.592241 | -99.592319 |
| [Ne] $3s^2$ | $^1S$ | -100.765362 | -100.767880 | -100.768268 | -100.768339 |
| [Ne] $3s^2 3p^1$ | $^2P$ | -101.341340 | -101.344430 | -101.344845 | -101.344910 |
| [Ne] $3s^2 3p^3$ | $^4S$ | -101.657754 | -101.660560 | -101.660972 | -101.661043 |
| Correlation | | T | Q | 5 | CBS |
| [Ne] $3s^2 3p^2$ | $^3P$ | -0.336020 | -0.386298 | -0.405726 | -0.428232 |
| [Ne] | $^1S$ | -0.232488 | -0.278592 | -0.296671 | -0.317884 |
| [Ne] $3s^1$ | $^2S$ | -0.246107 | -0.293177 | -0.311571 | -0.333091 |
| [Ne] $3s^2$ | $^1S$ | -0.298506 | -0.346684 | -0.365457 | -0.387362 |
| [Ne] $3s^2 3p^1$ | $^2P$ | -0.319161 | -0.368422 | -0.387552 | -0.409811 |
| [Ne] $3s^2 3p^3$ | $^4S$ | -0.351145 | -0.402192 | -0.421832 | -0.444501 |

TABLE IX: Total energy components of various states of the P atom using our ccECP[Ne]

| SCF | | T | Q | 5 | CBS |
|---|---|---|---|---|---|
| [Ne] $3s^2 3p^3$ | $^4S$ | -6.340560 | -6.340906 | -6.340875 | -6.340917 |
| [Ne] $3s^1$ | $^2S$ | -2.362967 | -2.362961 | -2.362981 | -2.363013 |
| [Ne] $3s^2$ | $^1S$ | -4.186007 | -4.185996 | -4.186002 | -4.186015 |
| [Ne] $3s^2 3p^1$ | $^2P$ | -5.265263 | -5.265481 | -5.265501 | -5.265510 |
| [Ne] $3s^2 3p^2$ | $^3P$ | -5.970169 | -5.970641 | -5.970646 | -5.970670 |
| [Ne] $3s^2 3p^4$ | $^3P$ | -6.320061 | -6.320225 | -6.320176 | -6.320236 |
| Correlation | | T | Q | 5 | CBS |
| [Ne] $3s^2 3p^3$ | $^4S$ | -0.112732 | -0.115948 | -0.116922 | -0.117781 |
| [Ne] $3s^1$ | $^2S$ | | | | |
| [Ne] $3s^2$ | $^1S$ | -0.053463 | -0.053785 | -0.053895 | -0.054008 |
| [Ne] $3s^2 3p^1$ | $^2P$ | -0.077685 | -0.078756 | -0.079108 | -0.079454 |
| [Ne] $3s^2 3p^2$ | $^3P$ | -0.097219 | -0.099311 | -0.099955 | -0.100534 |
| [Ne] $3s^2 3p^4$ | $^3P$ | -0.155101 | -0.161173 | -0.162879 | -0.164211 |

TABLE X: Total energy components of various states of the P atom using our ccECP[He]

| SCF | | T | Q | 5 | CBS |
|---|---|---|---|---|---|
| [Ne] $3s^2 3p^3$ | $^4S$ | -125.253282 | -125.258161 | -125.258394 | -125.258405 |
| [Ne] | $^1S$ | -118.899156 | -118.903679 | -118.903877 | -118.903886 |
| [Ne] $3s^1$ | $^2S$ | -121.271178 | -121.275661 | -121.275885 | -121.275897 |
| [Ne] $3s^2$ | $^1S$ | -123.100459 | -123.104903 | -123.105109 | -123.105119 |
| [Ne] $3s^2 3p^1$ | $^2P$ | -124.180512 | -124.185217 | -124.185449 | -124.185461 |
| [Ne] $3s^2 3p^2$ | $^3P$ | -124.884427 | -124.889414 | -124.889658 | -124.889670 |
| [Ne] $3s^2 3p^4$ | $^3P$ | -125.233338 | -125.238037 | -125.238254 | -125.238264 |
| **Correlation** | | **T** | **Q** | **5** | **CBS** |
| [Ne] $3s^2 3p^3$ | $^4S$ | -0.365923 | -0.418003 | -0.438225 | -0.461752 |
| [Ne] | $^1S$ | -0.233066 | -0.278627 | -0.296756 | -0.318285 |
| [Ne] $3s^1$ | $^2S$ | -0.247871 | -0.294566 | -0.313051 | -0.334912 |
| [Ne] $3s^2$ | $^1S$ | -0.306293 | -0.354270 | -0.373190 | -0.395491 |
| [Ne] $3s^2 3p^1$ | $^2P$ | -0.330315 | -0.379711 | -0.399104 | -0.421880 |
| [Ne] $3s^2 3p^2$ | $^3P$ | -0.349999 | -0.400799 | -0.420623 | -0.443787 |
| [Ne] $3s^2 3p^4$ | $^3P$ | -0.408274 | -0.463170 | -0.484121 | -0.508132 |

TABLE XI: Total energy components of various states of the S atom using our ccECP[Ne]

| SCF | | T | Q | 5 | CBS |
|---|---|---|---|---|---|
| [Ne] $3s^2 3p^4$ | $^3P$ | -9.917772 | -9.918088 | -9.918140 | -9.918156 |
| [Ne] $3s^1$ | $^2S$ | -3.199330 | -3.199320 | -3.199373 | -3.199413 |
| [Ne] $3s^2$ | $^1S$ | -5.787262 | -5.787214 | -5.787263 | -5.787312 |
| [Ne] $3s^2 3p^1$ | $^2P$ | -7.490378 | -7.490458 | -7.490604 | -7.490623 |
| [Ne] $3s^2 3p^2$ | $^3P$ | -8.745383 | -8.745651 | -8.745767 | -8.745853 |
| [Ne] $3s^2 3p^3$ | $^4S$ | -9.587305 | -9.587807 | -9.587895 | -9.587914 |
| [Ne] $3s^2 3p^5$ | $^2P$ | -9.951496 | -9.951654 | -9.951678 | -9.951687 |
| Correlation | | T | Q | 5 | CBS |
| [Ne] $3s^2 3p^4$ | $^3P$ | -0.165776 | -0.173557 | -0.175915 | -0.177994 |
| [Ne] $3s^1$ | $^2S$ | | | | |
| [Ne] $3s^2$ | $^1S$ | -0.058888 | -0.059247 | -0.059376 | -0.059518 |
| [Ne] $3s^2 3p^1$ | $^2P$ | -0.085847 | -0.087076 | -0.087513 | -0.087980 |
| [Ne] $3s^2 3p^2$ | $^3P$ | -0.107509 | -0.109937 | -0.110748 | -0.111559 |
| [Ne] $3s^2 3p^3$ | $^4S$ | -0.124018 | -0.127843 | -0.129087 | -0.130294 |
| [Ne] $3s^2 3p^5$ | $^2P$ | -0.203222 | -0.214387 | -0.217619 | -0.220276 |

TABLE XII: Total energy components of various states of the S atom using our ccECP[He]

| SCF | | T | Q | 5 | CBS |
|---|---|---|---|---|---|
| [Ne] $3s^2 3p^4$ | $^3P$ | -151.909927 | -151.916064 | -151.916369 | -151.916385 |
| [Ne] | $^1S$ | -141.960834 | -141.966569 | -141.966790 | -141.966799 |
| [Ne] $3s^1$ | $^2S$ | -145.177455 | -145.183135 | -145.183423 | -145.183438 |
| [Ne] $3s^2$ | $^1S$ | -147.778004 | -147.783595 | -147.783878 | -147.783893 |
| [Ne] $3s^2 3p^1$ | $^2P$ | -149.483717 | -149.489469 | -149.489861 | -149.489890 |
| [Ne] $3s^2 3p^2$ | $^3P$ | -150.738321 | -150.744306 | -150.744672 | -150.744696 |
| [Ne] $3s^2 3p^3$ | $^4S$ | -151.578352 | -151.584628 | -151.584970 | -151.584989 |
| [Ne] $3s^2 3p^5$ | $^2P$ | -151.943481 | -151.949466 | -151.949744 | -151.949757 |
| Correlation | | T | Q | 5 | CBS |
| [Ne] $3s^2 3p^4$ | $^3P$ | -0.420401 | -0.477685 | -0.499872 | -0.525628 |
| [Ne] | $^1S$ | -0.233065 | -0.278340 | -0.296665 | -0.318728 |
| [Ne] $3s^1$ | $^2S$ | -0.248757 | -0.295307 | -0.314039 | -0.336489 |
| [Ne] $3s^2$ | $^1S$ | -0.312562 | -0.360586 | -0.379826 | -0.402804 |
| [Ne] $3s^2 3p^1$ | $^2P$ | -0.339291 | -0.389051 | -0.408907 | -0.432544 |
| [Ne] $3s^2 3p^2$ | $^3P$ | -0.361203 | -0.412731 | -0.433178 | -0.457406 |
| [Ne] $3s^2 3p^3$ | $^4S$ | -0.378375 | -0.431623 | -0.452638 | -0.477427 |
| [Ne] $3s^2 3p^5$ | $^2P$ | -0.458354 | -0.518979 | -0.542040 | -0.568391 |

TABLE XIII: Total energy components of various states of the Cl atom using our ccECP[Ne]

| SCF | | T | Q | 5 | CBS |
|---|---|---|---|---|---|
| [Ne] $3s^2 3p^5$ | $^2P$ | -14.688897 | -14.689151 | -14.689385 | -14.689386 |
| [Ne] $3s^1$ | $^2S$ | -4.153414 | -4.153407 | -4.153487 | -4.153506 |
| [Ne] $3s^2$ | $^1S$ | -7.623920 | -7.623836 | -7.623936 | -7.623950 |
| [Ne] $3s^2 3p^1$ | $^2P$ | -10.068949 | -10.069158 | -10.069416 | -10.069416 |
| [Ne] $3s^2 3p^2$ | $^3P$ | -11.995324 | -11.995572 | -11.995854 | -11.995856 |
| [Ne] $3s^2 3p^3$ | $^4S$ | -13.435190 | -13.435587 | -13.435816 | -13.435820 |
| [Ne] $3s^2 3p^4$ | $^3P$ | -14.255149 | -14.255690 | -14.255918 | -14.256085 |
| [Ne] $3s^2 3p^6$ | $^1S$ | -14.784864 | -14.784943 | -14.785142 | -14.785146 |
| **Correlation** | | **T** | **Q** | **5** | **CBS** |
| [Ne] $3s^2 3p^5$ | $^2P$ | -0.214761 | -0.228169 | -0.232225 | -0.235794 |
| [Ne] $3s^1$ | $^2S$ | | | | |
| [Ne] $3s^2$ | $^1S$ | -0.064175 | -0.064536 | -0.064686 | -0.064870 |
| [Ne] $3s^2 3p^1$ | $^2P$ | -0.093905 | -0.095211 | -0.095684 | -0.096199 |
| [Ne] $3s^2 3p^2$ | $^3P$ | -0.117691 | -0.120313 | -0.121206 | -0.122119 |
| [Ne] $3s^2 3p^3$ | $^4S$ | -0.135384 | -0.139587 | -0.140982 | -0.142366 |
| [Ne] $3s^2 3p^4$ | $^3P$ | -0.179033 | -0.187874 | -0.190649 | -0.193217 |
| [Ne] $3s^2 3p^6$ | $^1S$ | -0.247496 | -0.264870 | -0.269980 | -0.274288 |

TABLE XIV: Total energy components of various states of the Cl atom using our ccECP[He]

| SCF | | T | Q | 5 | CBS |
|---|---|---|---|---|---|
| [Ne] $3s^2 3p^5$ | $^2P$ | -181.606009 | -181.611999 | -181.612377 | -181.612402 |
| [Ne] | $^1S$ | -166.876313 | -166.881725 | -166.882022 | -166.882039 |
| [Ne] $3s^1$ | $^2S$ | -171.052574 | -171.057971 | -171.058355 | -171.058385 |
| [Ne] $3s^2$ | $^1S$ | -174.540922 | -174.546208 | -174.546602 | -174.546634 |
| [Ne] $3s^2 3p^1$ | $^2P$ | -176.989287 | -176.994921 | -176.995449 | -176.995504 |
| [Ne] $3s^2 3p^2$ | $^3P$ | -178.914799 | -178.920519 | -178.921056 | -178.921111 |
| [Ne] $3s^2 3p^3$ | $^4S$ | -180.351450 | -180.357396 | -180.357852 | -180.357890 |
| [Ne] $3s^2 3p^4$ | $^3P$ | -181.172702 | -181.178912 | -181.179310 | -181.179337 |
| [Ne] $3s^2 3p^6$ | $^1S$ | -181.700830 | -181.706653 | -181.706998 | -181.707020 |
| Correlation | | T | Q | 5 | CBS |
| [Ne] $3s^2 3p^5$ | $^2P$ | -0.472345 | -0.535132 | -0.559372 | -0.587434 |
| [Ne] | $^1S$ | -0.234937 | -0.279240 | -0.297555 | -0.319976 |
| [Ne] $3s^1$ | $^2S$ | -0.251472 | -0.297158 | -0.315912 | -0.338747 |
| [Ne] $3s^2$ | $^1S$ | -0.320306 | -0.367597 | -0.386907 | -0.410321 |
| [Ne] $3s^2 3p^1$ | $^2P$ | -0.349504 | -0.398752 | -0.418757 | -0.442915 |
| [Ne] $3s^2 3p^2$ | $^3P$ | -0.373428 | -0.424710 | -0.445416 | -0.470303 |
| [Ne] $3s^2 3p^3$ | $^4S$ | -0.391882 | -0.445213 | -0.466621 | -0.492226 |
| [Ne] $3s^2 3p^4$ | $^3P$ | -0.435816 | -0.493986 | -0.516894 | -0.543868 |
| [Ne] $3s^2 3p^6$ | $^1S$ | -0.506041 | -0.572752 | -0.598045 | -0.626863 |

TABLE XV: Total energy components of various states of the Ar atom using our ccECP[Ne]

| SCF | | T | Q | 5 | CBS |
|---|---|---|---|---|---|
| [Ne] $3s^2 3p^6$ | $^1S$ | -20.778934 | -20.779555 | -20.779573 | -20.779601 |
| [Ne] $3s^1$ | $^2S$ | -5.207475 | -5.207483 | -5.207610 | -5.207618 |
| [Ne] $3s^2$ | $^1S$ | -9.665000 | -9.664896 | -9.665081 | -9.665103 |
| [Ne] $3s^2 3p^1$ | $^2P$ | -12.964117 | -12.964630 | -12.964915 | -12.964920 |
| [Ne] $3s^2 3p^2$ | $^3P$ | -15.676104 | -15.676707 | -15.677049 | -15.677055 |
| [Ne] $3s^2 3p^3$ | $^4S$ | -17.831518 | -17.832105 | -17.832395 | -17.832680 |
| [Ne] $3s^2 3p^4$ | $^3P$ | -19.266038 | -19.266814 | -19.266949 | -19.266979 |
| [Ne] $3s^2 3p^5$ | $^2P$ | -20.234894 | -20.235814 | -20.235893 | -20.235923 |
| Correlation | | T | Q | 5 | CBS |
| [Ne] $3s^2 3p^6$ | $^1S$ | -0.259079 | -0.279406 | -0.285173 | -0.289756 |
| [Ne] $3s^1$ | $^2S$ | | | | |
| [Ne] $3s^2$ | $^1S$ | -0.069503 | -0.069933 | -0.070038 | -0.070099 |
| [Ne] $3s^2 3p^1$ | $^2P$ | -0.101947 | -0.103367 | -0.103790 | -0.104156 |
| [Ne] $3s^2 3p^2$ | $^3P$ | -0.127850 | -0.130675 | -0.131528 | -0.132275 |
| [Ne] $3s^2 3p^3$ | $^4S$ | -0.146823 | -0.151385 | -0.152764 | -0.153973 |
| [Ne] $3s^2 3p^4$ | $^3P$ | -0.192939 | -0.202715 | -0.205588 | -0.208007 |
| [Ne] $3s^2 3p^5$ | $^2P$ | -0.229486 | -0.244616 | -0.248974 | -0.252528 |

TABLE XVI: Total energy components of various states of the Ar atom using our ccECP[He]

| SCF | | T | Q | 5 | CBS |
|---|---|---|---|---|---|
| [Ne] $3s^2 3p^6$ | $^1S$ | -214.882779 | -214.891228 | -214.891473 | -214.891481 |
| [Ne] | $^1S$ | -194.015736 | -194.023303 | -194.023467 | -194.023471 |
| [Ne] $3s^1$ | $^2S$ | -199.262254 | -199.269806 | -199.270110 | -199.270123 |
| [Ne] $3s^2$ | $^1S$ | -203.750624 | -203.758010 | -203.758366 | -203.758384 |
| [Ne] $3s^2 3p^1$ | $^2P$ | -207.059126 | -207.067196 | -207.067647 | -207.067674 |
| [Ne] $3s^2 3p^2$ | $^3P$ | -209.774739 | -209.782966 | -209.783460 | -209.783491 |
| [Ne] $3s^2 3p^3$ | $^4S$ | -211.929923 | -211.938199 | -211.938633 | -211.938657 |
| [Ne] $3s^2 3p^4$ | $^3P$ | -213.368960 | -213.377490 | -213.377782 | -213.377792 |
| [Ne] $3s^2 3p^5$ | $^2P$ | -214.339213 | -214.347933 | -214.348210 | -214.348219 |
| Correlation | | T | Q | 5 | CBS |
| [Ne] $3s^2 3p^6$ | $^1S$ | -0.516297 | -0.586767 | -0.613131 | -0.642806 |
| [Ne] | $^1S$ | -0.234846 | -0.279060 | -0.297392 | -0.319883 |
| [Ne] $3s^1$ | $^2S$ | -0.251903 | -0.297609 | -0.316402 | -0.339315 |
| [Ne] $3s^2$ | $^1S$ | -0.325612 | -0.373081 | -0.392439 | -0.415887 |
| [Ne] $3s^2 3p^1$ | $^2P$ | -0.356990 | -0.406593 | -0.426698 | -0.450934 |
| [Ne] $3s^2 3p^2$ | $^3P$ | -0.382642 | -0.434514 | -0.455381 | -0.480384 |
| [Ne] $3s^2 3p^3$ | $^4S$ | -0.402186 | -0.456407 | -0.478050 | -0.503818 |
| [Ne] $3s^2 3p^4$ | $^3P$ | -0.448215 | -0.507975 | -0.531290 | -0.558527 |
| [Ne] $3s^2 3p^5$ | $^2P$ | -0.485495 | -0.550750 | -0.575657 | -0.604203 |

## II. MOLECULAR DATA

TABLE XVII: All-electron (AE) UCCSD(T) Na2 ground state ($^1\Sigma_g$) binding parameters and potential energy surface along with the errors from uncorrelated core (UC) and ECPs. All energies in eV.

| Qty. | Exp. | AE | Discrepancies from AE | | | | | | |
|---|---|---|---|---|---|---|---|---|---|
| | | | UC | SBKJC | BFD | TN-DF | STU | ccECP[Ne] | ccECP[He] |
| Binding Parameters | | | | | | | | | |
| $D_e$(eV) | 0.737(13)$^{\dagger\ a}$ | 0.730(6) | -0.012(9) | -0.016(9) | -0.011(9) | -0.010(9) | -0.013(9) | 0.015(9) | -0.002(10) |
| $\omega_e$(cm$^{-1}$) | 139.9$^a$ | 146(3) | -10(5) | -11(5) | -10(5) | -10(5) | -10(5) | -1(5) | -1(5) |
| $r_e$(Å) | 3.079$^b$ | 3.069(18) | 0.116(28) | 0.103(28) | 0.099(28) | 0.094(28) | 0.098(28) | -0.007(26) | 0.005(29) |
| Potential Energy Surface | | | | | | | | | |
| U(2.20) | | -0.0369 | 0.1300 | 0.0868 | 0.0887 | 0.0806 | 0.0843 | -0.0460 | 0.00494 |
| U(2.45) | | -0.4296 | 0.0971 | 0.0773 | 0.0742 | 0.0686 | 0.0730 | -0.0288 | 0.00487 |
| U(2.70) | | -0.6443 | 0.0628 | 0.0557 | 0.0500 | 0.0464 | 0.0510 | -0.0201 | 0.00442 |
| U(2.95) | | -0.7324 | 0.0315 | 0.0322 | 0.0260 | 0.0241 | 0.0280 | -0.0152 | 0.00528 |
| U(3.20) | | -0.7350 | 0.0056 | 0.0104 | 0.0047 | 0.0043 | 0.0070 | -0.0133 | -0.00323 |
| U(3.45) | | -0.6841 | -0.0141 | -0.0081 | -0.0126 | -0.0125 | -0.0105 | -0.0134 | -0.00253 |

† Sum of experimental dissociation and zero-point energies

[a] Reference [1]

[b] Reference [2]

TABLE XVIII: All-electron (AE) UCCSD(T) NaO ground state ($^2\Sigma$) binding parameters and potential energy surface along with the errors from uncorrelated core (UC) and ECPs. All energies in eV.

| Qty. | Exp. | AE | Discrepancies from AE | | | | | | |
|---|---|---|---|---|---|---|---|---|---|
| | | | UC | SBKJC | BFD | TN-DF | STU | ccECP[Ne] | ccECP[He] |
| Binding Parameters | | | | | | | | | |
| $D_e$(eV) | 2.67[†] [a] | 2.52(2) | 0.05(3) | 0.06(2) | 0.02(3) | -0.00(2) | 0.01(2) | -0.02(3) | -0.01(3) |
| $\omega_e$(cm$^{-1}$) | 526[a] | 538(6) | -13(10) | -50(6) | -19(10) | -63(6) | -37(7) | -12(8) | 0(8) |
| $r_e$(Å) | 1.95[a] | 1.964(5) | 0.044(9) | -0.012(5) | 0.033(8) | -0.016(5) | 0.007(6) | 0.006(7) | 0.001(6) |
| Potential Energy Surface | | | | | | | | | |
| U(1.475) | | -0.0305 | 0.4054 | -0.7805 | 0.1843 | -0.8672 | -0.3741 | -0.0486 | 0.0252 |
| U(1.725) | | -2.1531 | 0.0936 | -0.1597 | 0.0563 | -0.1069 | -0.0414 | 0.0124 | 0.0134 |
| U(1.975) | | -2.4941 | -0.0390 | -0.0732 | -0.0169 | -0.0127 | -0.0181 | 0.0180 | 0.0090 |
| U(2.225) | | -2.2604 | -0.0964 | -0.0902 | -0.0640 | -0.0458 | -0.0472 | 0.0047 | 0.0068 |

[†] Sum of experimental dissociation and zero-point energies

[a] Reference [2]

## III. CL AND AR ALTERNATIVES

In Table XXXI, we share the alternative Ne-core ECP parameters for Cl and Ar which were generated with higher weights on the spectral component of the objective function. Additionally, the UCCSD(T) spectral errors and UCCSD(T) molecular errors from all-electron results are also provided. For Cl, the spectral errors are given in Table XXXII while the molecular errors are given in Figure 1 and Tables XXXIII and XXXIV. And for Ar, the spectral errors are given in Table XXXV while the molecular errors are given in Figure 2 and Table XXXVI. In the figures and tables, we have labeled these alternative ECPs as ccECP[Ne].S.

TABLE XIX: All-electron (AE) UCCSD(T) MgO ground state ($^1\Sigma^+$) binding parameters and potential energy surface along with the errors from uncorrelated core (UC) and ECPs. All energies in eV.

| Qty. | Exp. | AE | Discrepancies from AE | | | | | | |
|---|---|---|---|---|---|---|---|---|---|
| | | | UC | SBKJC | BFD | TN-DF | STU | ccECP[Ne] | ccECP[He] |
| Binding Parameters | | | | | | | | | |
| $D_e$(eV) | 2.5(2)$^{\dagger\ a}$ | 2.616(8) | 0.01(1) | 0.09(1) | 0.14(1) | -0.02(1) | 0.04(1) | -0.03(1) | 0.00(1) |
| $\omega_e$(cm$^{-1}$) | 785.2$^b$ | 780(6) | -14(8) | -39(8) | -7(8) | -43(9) | -17(8) | -33(8) | -1(9) |
| $r_e$(Å) | 1.749$^c$ | 1.738(2) | 0.017(3) | 0.005(3) | -0.020(3) | 0.004(4) | -0.007(3) | 0.007(3) | 0.000(3) |
| Potential Energy Surface | | | | | | | | | |
| U(1.4) | | -0.0876 | 0.2135 | -0.2493 | -0.6121 | -0.2685 | -0.3327 | -0.1149 | 0.0013 |
| U(1.5) | | -1.5908 | 0.1230 | -0.0830 | -0.3654 | -0.0738 | -0.1695 | -0.0054 | 0.0013 |
| U(1.6) | | -2.3414 | 0.0581 | -0.0189 | -0.2259 | 0.0012 | -0.0844 | 0.0319 | 0.0016 |
| U(1.7) | | -2.6140 | 0.0113 | -0.0037 | -0.1484 | 0.0203 | -0.0423 | 0.0368 | 0.0019 |
| U(1.8) | | -2.5929 | -0.0230 | -0.0132 | -0.1096 | 0.0124 | -0.0278 | 0.0239 | 0.0014 |

† Sum of experimental dissociation and zero-point energies

[a] Reference [3]

[b] Reference [4]

[c] Reference [2]

TABLE XX: All-electron (AE) UCCSD(T) Al2 ground state ($^3\Sigma_g$) binding parameters and potential energy surface along with the errors from uncorrelated core (UC) and ECPs. All energies in eV.

| Qty. | Exp. | AE | Discrepancies from AE | | | | | | |
|---|---|---|---|---|---|---|---|---|---|
| | | | UC | SBKJC | BFD | TN-DF | STU | ccECP[Ne] | ccECP[He] |
| Binding Parameters | | | | | | | | | |
| $D_e$(eV) | 1.34(13)[†] [a] | 1.423(3) | 0.002(5) | 0.014(5) | 0.035(5) | 0.010(5) | 0.048(5) | 0.009(5) | 0.003(5) |
| $\omega_e$(cm$^{-1}$) | 285.8[b] | 285(1) | -1(2) | 0(2) | 2(2) | -1(2) | 6(2) | -1(2) | 0(2) |
| $r_e$(Å) | 2.701[c] | 2.692(3) | 0.014(4) | 0.005(4) | -0.004(4) | 0.004(4) | -0.021(4) | -0.005(4) | -0.000(4) |
| Potential Energy Surface | | | | | | | | | |
| U(2.1) | | 0.0717 | 0.0817 | 0.0101 | -0.0473 | -0.0009 | -0.1253 | 0.0103 | -0.0034 |
| U(2.3) | | -0.9124 | 0.0392 | 0.0002 | -0.0409 | -0.0007 | -0.0900 | 0.0039 | -0.0035 |
| U(2.5) | | -1.3265 | 0.0129 | -0.0094 | -0.0383 | -0.0063 | -0.0657 | -0.0043 | -0.0034 |
| U(2.7) | | -1.4265 | -0.0023 | -0.0154 | -0.0359 | -0.0113 | -0.0477 | -0.0102 | -0.0033 |
| U(2.9) | | -1.3609 | -0.0102 | -0.0177 | -0.0326 | -0.0138 | -0.0335 | -0.0129 | -0.0031 |

[†] Sum of experimental dissociation and zero-point energies

[a] Reference [3]

[b] Reference [4]

[c] Reference [5]

TABLE XXI: All-electron (AE) UCCSD(T) AlO ground state ($^2\Sigma$) binding parameters and potential energy surface along with the errors from uncorrelated core (UC) and ECPs. All energies in eV.

| Qty. | Exp. | AE | Discrepancies from AE | | | | | | |
|---|---|---|---|---|---|---|---|---|---|
| | | | UC | SBKJC | BFD | TN-DF | STU | ccECP[Ne] | ccECP[He] |
| Potential Energy Surface | | | | | | | | | |
| $D_e$(eV) | 5.26(9)[†] [a] | 5.28(1) | -0.02(1) | 0.01(1) | 0.06(1) | -0.24(1) | 0.07(1) | 0.04(1) | -0.01(1) |
| $\omega_e$(cm$^{-1}$) | 979.5[b] | 1028(5) | -4(7) | -36(6) | -26(6) | -90(6) | -12(6) | -36(6) | 6(6) |
| $r_e$(Å) | 1.618[c] | 1.611(2) | 0.007(3) | 0.004(2) | -0.002(2) | 0.021(2) | -0.009(2) | 0.004(2) | -0.003(2) |
| Potential Energy Surface | | | | | | | | | |
| U(1.22) | | 1.3650 | 0.2753 | -0.4581 | -0.6482 | -0.3602 | -0.7520 | -0.4704 | -0.0202 |
| U(1.32) | | -2.3179 | 0.1699 | -0.1595 | -0.3070 | 0.1097 | -0.4055 | -0.1652 | -0.0153 |
| U(1.42) | | -4.2349 | 0.0980 | -0.0432 | -0.1495 | 0.2764 | -0.2200 | -0.0448 | -0.0104 |
| U(1.52) | | -5.0781 | 0.0494 | -0.0084 | -0.0800 | 0.2913 | -0.1202 | -0.0064 | -0.0064 |
| U(1.62) | | -5.2884 | 0.0179 | -0.0056 | -0.0508 | 0.2437 | -0.0654 | -0.0005 | 0.0209 |

[†] Sum of experimental dissociation and zero-point energies

[a] Reference [3]

[b] Reference [4]

[c] Reference [2]

TABLE XXII: All-electron (AE) UCCSD(T) Si2 ground state ($^3\Sigma_g$) binding parameters and potential energy surface along with the errors from uncorrelated core (UC) and ECPs. All energies in eV.

| Qty. | Exp. | AE | Discrepancies from AE | | | | | | |
|---|---|---|---|---|---|---|---|---|---|
| | | | UC | SBKJC | BFD | TN-DF | STU | ccECP[Ne] | ccECP[He] |
| Binding Parameters | | | | | | | | | |
| $D_e$(eV) | 3.239[†] [a] | 3.258(4) | -0.012(6) | -0.004(6) | 0.015(6) | 0.007(6) | 0.085(6) | 0.006(6) | 0.011(6) |
| $\omega_e$(cm$^{-1}$) | 489.7[a] | 506(2) | -3(3) | -4(3) | -2(3) | -4(3) | 9(3) | -4(3) | 0(3) |
| $r_e$(Å) | 2.246[b] | 2.242(2) | 0.009(2) | 0.004(3) | -0.004(3) | 0.001(3) | -0.023(2) | 0.003(2) | 0.001(3) |
| Potential Energy Surface | | | | | | | | | |
| U(1.750) | | 0.1044 | 0.1444 | -0.0001 | -0.1319 | -0.0554 | -0.3778 | -0.0134 | -0.0011 |
| U(1.875) | | -1.7121 | 0.0935 | 0.0145 | -0.0711 | -0.0221 | -0.2633 | 0.0072 | -0.0052 |
| U(2.000) | | -2.7013 | 0.0563 | 0.0139 | -0.0401 | -0.0102 | -0.1822 | 0.0112 | -0.0060 |
| U(2.125) | | -3.1540 | 0.0298 | 0.0083 | -0.0243 | -0.0079 | -0.1236 | 0.0087 | -0.0076 |
| U(2.250) | | -3.2654 | 0.0113 | 0.0023 | -0.0159 | -0.0089 | -0.0804 | 0.0047 | -0.0142 |
| U(2.375) | | -3.1650 | -0.0013 | -0.0025 | -0.0110 | -0.0103 | -0.0481 | 0.0010 | -0.0138 |

i

[†] Sum of experimental dissociation and zero-point energies

[a] Reference [1]

[b] Reference [2]

TABLE XXIII: All-electron (AE) UCCSD(T) SiO ground state ($^1\Sigma$) binding parameters and potential energy surface along with the errors from uncorrelated core (UC) and ECPs. All energies in eV.

| Qty. | Exp. | AE | Discrepancies from AE | | | | | | |
|---|---|---|---|---|---|---|---|---|---|
| | | | UC | SBKJC | BFD | TN-DF | STU | ccECP[Ne] | ccECP[He] |
| Binding Parameters | | | | | | | | | |
| $D_e$(eV) | 8.313(87)$^{\dagger\ a}$ | 8.33(2) | -0.04(2) | -0.02(2) | 0.02(2) | -0.16(2) | 0.10(2) | 0.01(2) | 0.01(2) |
| $\omega_e$(cm$^{-1}$) | 1259$^a$ | 1278(7) | -6(10) | -24(8) | -25(8) | -52(8) | -1(9) | -21(9) | 1(10) |
| $r_e$(Å) | 1.510$^b$ | 1.509(2) | 0.005(3) | 0.000(2) | -0.004(2) | 0.005(2) | -0.013(2) | -0.001(2) | 0.000(2) |
| Potential Energy Surface | | | | | | | | | |
| U(1.15) | | -0.1504 | 0.2614 | -0.3946 | -0.7175 | -0.3682 | -0.9623 | -0.3928 | -0.0212 |
| U(1.25) | | -4.9302 | 0.1693 | -0.1252 | -0.3053 | 0.0205 | -0.5351 | -0.1373 | -0.0186 |
| U(1.35) | | -7.2762 | 0.1053 | -0.0272 | -0.1258 | 0.1447 | -0.2942 | -0.0390 | -0.0146 |
| U(1.45) | | -8.1833 | 0.0609 | 0.0012 | -0.0498 | 0.1551 | -0.1536 | -0.0055 | -0.0111 |
| U(1.55) | | -8.2557 | 0.0300 | 0.0037 | -0.0194 | 0.1264 | -0.0695 | 0.0022 | -0.0086 |
| U(1.65) | | -7.8612 | 0.0084 | -0.0019 | -0.0084 | 0.0913 | -0.0184 | 0.0005 | -0.0070 |

$^\dagger$ Sum of experimental dissociation and zero-point energies

$^a$ Reference [1]

$^b$ Reference [6]

TABLE XXIV: All-electron (AE) UCCSD(T) P2 ground state ($^1\Sigma_g$) binding parameters and potential energy surface along with the errors from uncorrelated core (UC) and ECPs. All energies in eV.

| Qty. | Exp. | AE | Discrepancies from AE | | | | | | |
|---|---|---|---|---|---|---|---|---|---|
| | | | UC | SBKJC | BFD | TN-DF | STU | ccECP[Ne] | ccECP[He] |
| Binding Parameters | | | | | | | | | |
| $D_e$(eV) | 5.082(22)$^{\dagger\ a}$ | 4.96(2) | -0.03(2) | -0.06(2) | -0.03(2) | -0.03(2) | -0.13(2) | -0.05(2) | 0.01(2) |
| $\omega_e$(cm$^{-1}$) | 769.5$^a$ | 769(8) | -7(10) | -11(11) | -7(11) | -8(11) | -15(11) | -9(11) | 0(11) |
| $r_e$(Å) | 1.893$^b$ | 1.887(3) | 0.008(4) | 0.005(4) | -0.004(4) | 0.001(4) | 0.002(4) | 0.003(4) | 0.001(4) |
| Potential Energy Surface | | | | | | | | | |
| U(1.55) | | -1.2900 | 0.1760 | 0.0708 | -0.1612 | -0.0236 | 0.0331 | 0.0354 | -0.0046 |
| U(1.65) | | -3.4331 | 0.1197 | 0.0846 | -0.0555 | 0.0191 | 0.1027 | 0.0571 | -0.0093 |
| U(1.75) | | -4.5340 | 0.0767 | 0.0774 | -0.0006 | 0.0330 | 0.1281 | 0.0580 | -0.0122 |
| U(1.85) | | -4.9504 | 0.0442 | 0.0629 | 0.0263 | 0.0336 | 0.1311 | 0.0505 | -0.0122 |
| U(1.95) | | -4.9286 | 0.0197 | 0.0475 | 0.0379 | 0.0288 | 0.1234 | 0.0406 | -0.0130 |

$^\dagger$ Sum of experimental dissociation and zero-point energies

$^a$ Reference [1]

$^b$ Reference [2]

TABLE XXV: All-electron (AE) UCCSD(T) PO ground state ($^2\Pi$) binding parameters and potential energy surface along with the errors from uncorrelated core (UC) and ECPs. All energies in eV.

| Qty. | Exp. | AE | Discrepancies from AE | | | | | | |
|---|---|---|---|---|---|---|---|---|---|
| | | | UC | SBKJC | BFD | TN-DF | STU | ccECP[Ne] | ccECP[He] |
| Binding Parameters | | | | | | | | | |
| $D_e$(eV) | 6.16(13)$^{\dagger\ a}$ | 6.14(1) | -0.03(2) | -0.03(2) | -0.01(2) | -0.10(2) | -0.09(2) | -0.03(2) | 0.01(2) |
| $\omega_e$(cm$^{-1}$) | 1233.3$^b$ | 1249(7) | -7(10) | -11(11) | -11(11) | -19(11) | -14(11) | -9(11) | 0(10) |
| $r_e$(Å) | 1.476$^c$ | 1.472(1) | 0.004(2) | 0.001(2) | -0.004(2) | 0.003(2) | -0.002(2) | 0.000(2) | 0.000(2) |
| Potential Energy Surface | | | | | | | | | |
| U(1.2) | | -1.9498 | 0.1467 | -0.0306 | -0.2437 | 0.0845 | -0.1000 | -0.0560 | -0.0233 |
| U(1.3) | | -4.8025 | 0.0901 | 0.0229 | -0.0790 | 0.1248 | 0.0246 | 0.0052 | -0.0156 |
| U(1.4) | | -5.9524 | 0.0514 | 0.0319 | -0.0108 | 0.1154 | 0.0732 | 0.0235 | -0.0101 |
| U(1.5) | | -6.1369 | 0.0246 | 0.0270 | 0.0159 | 0.0944 | 0.0882 | 0.0258 | -0.0068 |
| U(1.6) | | -5.7942 | 0.0059 | 0.0192 | 0.0248 | 0.0739 | 0.0881 | 0.0225 | -0.0050 |

† Sum of experimental dissociation and zero-point energies

[a] Reference [1]

[b] Reference [4]

[c] Reference [2]

TABLE XXVI: All-electron (AE) UCCSD(T) S2 ground state ($^3\Sigma_g$) binding parameters and potential energy surface along with the errors from uncorrelated core (UC) and ECPs. All energies in eV.

| Qty. | Exp. | AE | Discrepancies from AE | | | | | | |
|---|---|---|---|---|---|---|---|---|---|
| | | | UC | SBKJC | BFD | TN-DF | STU | ccECP[Ne] | ccECP[He] |
| Binding Parameters | | | | | | | | | |
| $D_e$(eV) | 4.408(3)$^{\dagger\ a}$ | 4.429(7) | -0.02(1) | 0.00(1) | 0.01(1) | 0.01(1) | 0.12(1) | -0.02(1) | 0.02(1) |
| $\omega_e$(cm$^{-1}$) | 699.5$^a$ | 717(3) | -4(5) | -3(5) | -3(5) | -3(5) | 17(5) | -5(5) | 1(5) |
| $r_e$(Å) | 1.889$^b$ | 1.886(2) | 0.006(2) | 0.001(2) | -0.006(2) | 0.001(2) | -0.025(2) | 0.003(2) | -0.001(2) |
| Potential Energy Surface | | | | | | | | | |
| U(1.5) | | 0.3808 | 0.1600 | -0.0256 | -0.2756 | -0.0329 | -0.7207 | 0.0272 | -0.0263 |
| U(1.6) | | -2.2587 | 0.1076 | -0.0055 | -0.1444 | -0.0117 | -0.4797 | 0.0354 | -0.0258 |
| U(1.7) | | -3.6725 | 0.0692 | -0.0013 | -0.0705 | -0.0081 | -0.3102 | 0.0306 | -0.0241 |
| U(1.8) | | -4.3034 | 0.0412 | -0.0023 | -0.0284 | -0.0100 | -0.1899 | 0.0223 | -0.0221 |
| U(1.9) | | -4.4421 | 0.0211 | -0.0041 | -0.0043 | -0.0127 | -0.1042 | 0.0143 | -0.0199 |
| U(2.0) | | -4.2789 | 0.0066 | -0.0056 | 0.0094 | -0.0147 | -0.0430 | 0.0079 | -0.0177 |

$^\dagger$ Sum of experimental dissociation and zero-point energies

$^a$ Reference [1]

$^b$ Reference [2]

TABLE XXVII: All-electron (AE) UCCSD(T) SO ground state ($^3\Sigma$) binding parameters and potential energy surface along with the errors from uncorrelated core (UC) and ECPs. All energies in eV.

| Qty. | Exp. | AE | Discrepancies from AE | | | | | | |
|---|---|---|---|---|---|---|---|---|---|
| | | | UC | SBKJC | BFD | TN-DF | STU | ccECP[Ne] | ccECP[He] |
| Binding Parameters | | | | | | | | | |
| $D_e$(eV) | 5.421(13)[†] [a] | 5.412(7) | -0.021(9) | -0.01(1) | 0.02(1) | -0.06(1) | 0.03(1) | -0.02(1) | 0.01(1) |
| $\omega_e$(cm$^{-1}$) | 1119[a] | 1165(3) | -5(4) | -6(5) | -7(5) | -13(5) | 6(5) | -7(5) | 0(5) |
| $r_e$(Å) | 1.481[b] | 1.4772(8) | 0.004(1) | 0.001(1) | -0.005(1) | 0.004(1) | -0.012(1) | 0.001(1) | 0.000(1) |
| Potential Energy Surface | | | | | | | | | |
| U(1.15) | | 0.7445 | 0.1464 | -0.0520 | -0.4014 | 0.1084 | -0.5759 | -0.0397 | -0.0339 |
| U(1.25) | | -3.0835 | 0.0913 | -0.0052 | -0.1843 | 0.1147 | -0.3000 | 0.0055 | -0.0193 |
| U(1.35) | | -4.8278 | 0.0536 | 0.0053 | -0.0830 | 0.0916 | -0.1382 | 0.0164 | -0.0103 |
| U(1.45) | | -5.3932 | 0.0277 | 0.0047 | -0.0352 | 0.0667 | -0.0429 | 0.0152 | -0.0057 |
| U(1.55) | | -5.3060 | 0.0098 | 0.0014 | -0.0128 | 0.0464 | 0.0128 | 0.0101 | -0.0039 |

[†] Sum of experimental dissociation and zero-point energies

[a] Reference [1]

[b] Reference [2]

TABLE XXVIII: All-electron (AE) UCCSD(T) Cl2 ground state ($^1\Sigma_g$) binding parameters and potential energy surface along with the errors from uncorrelated core (UC) and ECPS. All energies in eV.

| Qty. | Exp. | AE | Discrepancies from AE | | | | | | |
|---|---|---|---|---|---|---|---|---|---|
| | | | UC | SBKJC | BFD | TN-DF | STU | ccECP[Ne] | ccECP[He] |
| Binding Parameters | | | | | | | | | |
| $D_e$(eV) | 2.5143(4)$^{\dagger\ a}$ | 2.526(9) | -0.01(1) | -0.01(1) | 0.02(1) | -0.01(1) | 0.04(1) | -0.01(1) | 0.01(1) |
| $\omega_e$(cm$^{-1}$) | 559.6$^a$ | 533(5) | -3(7) | 0(7) | 1(7) | -2(7) | 12(8) | -2(7) | 1(7) |
| $r_e$(Å) | 1.988$^b$ | 1.987(3) | 0.005(5) | -0.001(5) | -0.009(5) | 0.002(5) | -0.025(5) | 0.002(5) | 0.000(5) |
| Potential Energy Surface | | | | | | | | | |
| U(1.6) | | 0.5063 | 0.0825 | -0.0122 | -0.2120 | 0.0335 | -0.4174 | -0.0025 | -0.0102 |
| U(1.7) | | -1.1542 | 0.0534 | -0.0036 | -0.1263 | 0.0279 | -0.2635 | 0.0070 | -0.0112 |
| U(1.8) | | -2.0502 | 0.0325 | 0.0011 | -0.0736 | 0.0215 | -0.1556 | 0.0110 | -0.0117 |
| U(1.9) | | -2.4538 | 0.0174 | 0.0037 | -0.0409 | 0.0162 | -0.0796 | 0.0125 | -0.0117 |
| U(2.0) | | -2.5435 | 0.0066 | 0.0053 | -0.0208 | 0.0120 | -0.0263 | 0.0127 | -0.0114 |
| U(2.1) | | -2.4387 | -0.0011 | 0.0059 | -0.0085 | 0.0088 | 0.0102 | 0.0121 | -0.0109 |

$^\dagger$ Sum of experimental dissociation and zero-point energies

$^a$ Reference [1]

$^b$ Reference [2]

TABLE XXIX: All-electron (AE) UCCSD(T) ClO ground state ($^2\Pi$) binding parameters and potential energy surface along with the errors from uncorrelated core (UC) and ECPS. All energies in eV.

| Qty. | Exp. | AE | Discrepancies from AE | | | | | | |
|---|---|---|---|---|---|---|---|---|---|
| | | | UC | SBKJC | BFD | TN-DF | STU | ccECP[Ne] | ccECP[He] |
| Binding Parameters | | | | | | | | | |
| $D_e$(eV) | 2.802(1)$^{\dagger\ a}$ | 2.753(5) | -0.009(7) | -0.012(7) | 0.035(7) | -0.060(7) | -0.026(8) | -0.016(7) | -0.001(7) |
| $\omega_e$(cm$^{-1}$) | 839.4$^a$ | 851(3) | -3(4) | -4(4) | 0(4) | -13(4) | -4(4) | -6(4) | -2(4) |
| $r_e$(Å) | 1.596$^b$ | 1.564(1) | 0.004(1) | 0.001(2) | -0.008(2) | 0.007(2) | -0.007(2) | 0.001(2) | 0.001(2) |
| Potential Energy Surface | | | | | | | | | |
| U(1.17) | | 3.2728 | 0.1081 | -0.1807 | -0.5878 | 0.0054 | -0.5093 | -0.0260 | -0.0119 |
| U(1.27) | | -0.1726 | 0.0674 | -0.1125 | -0.3375 | 0.0232 | -0.2738 | 0.0076 | -0.0002 |
| U(1.37) | | -1.8723 | 0.0400 | -0.0694 | -0.1919 | 0.0256 | -0.1525 | 0.0172 | 0.0038 |
| U(1.47) | | -2.5904 | 0.0215 | -0.0423 | -0.1080 | 0.0244 | -0.0766 | 0.0174 | 0.0034 |
| U(1.57) | | -2.7621 | 0.0089 | -0.0259 | -0.0592 | 0.0224 | -0.0219 | 0.0146 | 0.0012 |
| U(1.67) | | -2.6326 | 0.0002 | -0.0156 | -0.0297 | 0.0205 | 0.0167 | 0.0114 | -0.0010 |

† Sum of experimental dissociation and zero-point energies

[a] Reference [1]

[b] Reference [6]

TABLE XXX: All-electron (AE) UCCSD(T) ArH+ ground state ($^1\Sigma$) binding parameters and potential energy surface along with the errors from uncorrelated core (UC) and ECPs. All energies in eV.

| Qty. | Exp. | AE | Discrepancies from AE | | | | | | |
|---|---|---|---|---|---|---|---|---|---|
| | | | UC | SBKJC | BFD | TN-DF | STU | ccECP[Ne] | ccECP[He] |
| Binding Parameters | | | | | | | | | |
| $D_e$(eV) | 4.059[†] [a] | 4.072(4) | 0.004(6) | -0.001(6) | 0.026(6) | 0.001(6) | -0.015(6) | 0.000(6) | 0.001(6) |
| $\omega_e$(cm$^{-1}$) | 2723[a] | 2728(18) | -1(26) | 2(25) | 1(25) | 0(26) | -8(25) | -1(25) | 2(26) |
| $r_e$(Å) | 1.286[a] | 1.282(1) | 0.001(1) | 0.000(1) | -0.004(1) | 0.001(1) | -0.002(1) | 0.000(1) | 0.000(1) |
| Potential Energy Surface | | | | | | | | | |
| U(0.9) | | 0.4748 | 0.0307 | 0.0081 | -0.1533 | 0.0213 | -0.0770 | -0.0033 | 0.0020 |
| U(1.0) | | -2.1495 | 0.0160 | 0.0067 | -0.0913 | 0.0137 | -0.0282 | 0.0014 | 0.0006 |
| U(1.1) | | -3.4435 | 0.0062 | 0.0041 | -0.0562 | 0.0064 | -0.0030 | 0.0014 | 0.0004 |
| U(1.2) | | -3.9723 | -0.0003 | 0.0022 | -0.0361 | 0.0012 | 0.0099 | 0.0004 | 0.0008 |
| U(1.3) | | -4.0653 | -0.0045 | 0.0013 | -0.0244 | -0.0018 | 0.0161 | -0.0006 | 0.0015 |
| U(1.4) | | -3.9164 | -0.0072 | 0.0012 | -0.0174 | -0.0035 | 0.0186 | -0.0013 | 0.0022 |

[†] Sum of experimental dissociation and zero-point energies

[a] Reference [7]

TABLE XXXI: Parameter values for Cl and Ar ccECP[Ne].S potentials. The highest $l$ value corresponds to the local channel.

| Atom | $Z_{\text{eff}}$ | $l$ | $n_{l,k}$ | $\alpha_{l,k}$ | $\beta_{l,k}$ |
|---|---|---|---|---|---|
| Cl | 7 | 0 | 2 | 17.23708573 | 6.50888648 |
| | | 0 | 2 | 4.31148447 | 46.76346700 |
| | | 1 | 2 | 11.38275704 | 2.99464770 |
| | | 1 | 2 | 3.83218762 | 28.01703410 |
| | | 2 | 1 | 22.71655173 | 7.00000000 |
| | | 2 | 3 | 78.57185685 | 159.01586213 |
| | | 2 | 2 | 7.47352436 | -15.65310650 |
| Ar | 8 | 0 | 2 | 26.06800734 | 7.67833187 |
| | | 0 | 2 | 5.17516183 | 60.31303710 |
| | | 1 | 2 | 17.09350095 | 3.47705723 |
| | | 1 | 2 | 4.64108131 | 36.47236220 |
| | | 2 | 1 | 8.98034652 | 8.00000000 |
| | | 2 | 3 | 26.23635698 | 71.84277216 |
| | | 2 | 2 | 7.10917092 | -22.13000430 |

TABLE XXXII: All-electron (AE) UCCSD(T) ionization potentials and electron affinity of Cl along with the errors from ccECP[Ne].S. The uncontracted aug-cc-pCV5Z basis was used for all calculations. All values in eV. See Tab. V in main text for further description.

| Qty. | AE | Discrepancy from AE<br>ccECP[Ne].S |
|---|---|---|
| IP(I) | 12.9388 | -0.0427 |
| IP(II) | 23.7309 | -0.0830 |
| IP(III) | 39.6980 | 0.0233 |
| IP(IV) | 53.1811 | -0.0321 |
| IP(V) | 67.6102 | -0.1362 |
| IP(VI) | 96.8961 | -0.1292 |
| IP(VII) | 114.2079 | -0.4249 |
| EA | 3.6210 | -0.0184 |
| AMAD | | 0.1112 |
| LMAD | | 0.0480 |
| MARE | | 0.0025 |

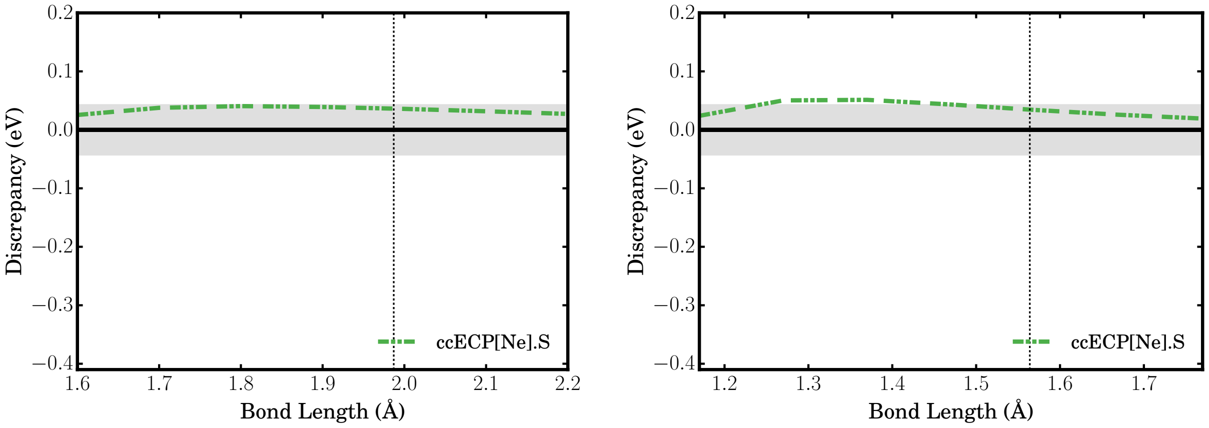


(a) Cl2 binding curve discrepancies

(b) ClO binding curve discrepancies

FIG. 1: Binding energy discrepancies for (a) Cl2 and (b) ClO molecules in their ground states $^1\Sigma_g$ and $^2\Pi$, respectively. The binding curves are relative to the AE UCCSD(T) binding curve. The shaded region indicates a discrepancy of chemical accuracy in either direction.

TABLE XXXIII: All-electron (AE) UCCSD(T) Cl2 ground state ($^1\Sigma_g$) binding parameters and potential energy surface along with the errors from ccECP[Ne].S. All energies in eV.

| Qty. | AE | Discrepancy from AE ccECP[Ne].S |
|---|---|---|
| Binding Parameters | | |
| $D_e$(eV) | 2.526(9) | -0.04(1) |
| $\omega_e$(cm$^{-1}$) | 533(5) | -5(7) |
| $r_e$(Å) | 1.987(3) | 0.002(5) |
| Potential Energy Surface | | |
| U(1.6) | 0.5063 | 0.0254 |
| U(1.7) | -1.1542 | 0.0377 |
| U(1.8) | -2.0502 | 0.0406 |
| U(1.9) | -2.4538 | 0.0391 |
| U(2.0) | -2.5435 | 0.0358 |
| U(2.1) | -2.4387 | 0.0317 |

TABLE XXXIV: All-electron (AE) UCCSD(T) ClO ground state ($^2\Pi$) binding parameters and potential energy surface along with the errors from ccECP[Ne].S. All energies in eV.

| Qty. | AE | Discrepancy from AE ccECP[Ne].S |
|---|---|---|
| Binding Parameters | | |
| $D_e$(eV) | 2.753(5) | -0.036(7) |
| $\omega_e$(cm$^{-1}$) | 850(3) | -10(4) |
| $r_e$(Å) | 1.564(1) | 0.003(2) |
| Potential Energy Surface | | |
| U(1.17) | 3.2728 | 0.0240 |
| U(1.27) | -0.1726 | 0.0503 |
| U(1.37) | -1.8723 | 0.0513 |
| U(1.47) | -2.5904 | 0.0433 |
| U(1.57) | -2.7621 | 0.0340 |
| U(1.67) | -2.6326 | 0.0258 |

FIG. 2: Binding energy discrepancies for the ArH+ molecule in its ground state $^1\Sigma$. The binding curves are relative to the AE UCCSD(T) binding curve. The shaded region indicates a discrepancy of chemical accuracy in either direction.

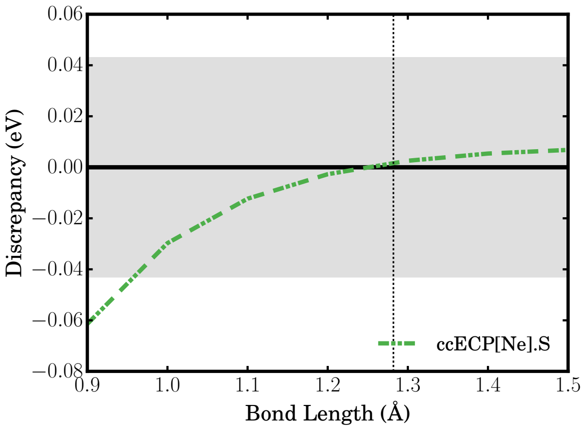

TABLE XXXV: All-electron (AE) UCCSD(T) ionization potentials and electron affinity of Ar along with the errors from ccECP[Ne].S. The uncontracted aug-cc-pCV5Z basis was used for all calculations. All values in eV. See Tab. V in main text for further description.

| Qty. | AE | Discrepancy from AE |
|---|---|---|
| | | ccECP[Ne].S |
| IP(I) | 15.7829 | 0.0202 |
| IP(II) | 27.6005 | -0.0126 |
| IP(III) | 40.6121 | -0.0862 |
| IP(IV) | 59.2804 | 0.0239 |
| IP(V) | 74.7437 | -0.1283 |
| IP(VI) | 91.1085 | -0.3698 |
| IP(VII) | 124.3356 | -0.1401 |
| IP(VIII) | 143.4706 | -0.5716 |
| AMAD | | 0.1112 |
| LMAD | | 0.0480 |
| MARE | | 0.0025 |

TABLE XXXVI: All-electron (AE) UCCSD(T) ArH+ ground state ($^1\Sigma$) binding parameters and potential energy surface along with the errors from ccECP[Ne].S. All energies in eV.

| Qty. | AE | Discrepancy from AE<br>ccECP[Ne].S |
|---|---|---|
| Binding Parameters | | |
| $D_e$(eV) | 4.072(4) | -0.002(6) |
| $\omega_e$(cm$^{-1}$) | 2728(18) | -2(25) |
| $r_e$(Å) | 1.282(1) | -0.002(1) |
| Potential Energy Surface | | |
| U(0.9) | 0.4748 | -0.0614 |
| U(1.0) | -2.1495 | -0.0297 |
| U(1.1) | -3.4435 | -0.0123 |
| U(1.2) | -3.9723 | -0.0027 |
| U(1.3) | -4.0653 | 0.0026 |
| U(1.4) | -3.9164 | 0.0054 |

[1] D. Feller and K. A. Peterson, The Journal of chemical physics **110**, 8384 (1999).

[2] K. Huber and G. Herzbery, Molecular spectra and molecular structure: IV. Constants of diatomic molecule (Van Nostrand Reinhold Co., 1979).

[3] R. D. J. III, NIST Computational Chemistry Comparison and Benchmark Database NIST Standard Reference Database Number 101 Release 19, [Online]. Available: `http://cccbdb.nist.gov/` [2018, April 19]. National Institute of Standards and Technology, Gaithersburg, MD. (2018).

[4] K. K. Irikura, Journal of physical and chemical reference data **36**, 389 (2007).

[5] Z. Fu, G. W. Lemire, G. A. Bishea, and M. D. Morse, The Journal of Chemical Physics **93**, 8420 (1990).

[6] F. J. Lovas, E. Tiemann, J. S. Coursey, S. A. Kotochigova, J. Chang, K. Olsen, and R. A. Dragoset, NIST Diatomic Spectral Database 114, [Online]. Available: `www.physics.nist.gov/PhysRefData/MolSpec/Diatomic/index.html` [2005, November]. Institut fr Quantenoptik, Universitt Hannover, Hannover, Germany (2005).

[7] P. Rosmus, Theoretica chimica acta **51**, 359 (1979).
